# Supplementary material for: Improved Equation of State for Finite-Temperature Spin-Polarized Electron Liquids on the Basis of Singwi-Tosi-Land-Sjolander Approximation
Source: arXiv:1612.09037 source file (2016-12-29)
Supplement: Supplementary file 1 [file STLS_SM_1229.pdf]

# Supplemental Material for Improved Equation of State for Finite-Temperature Spin-Polarized Electron Liquids on the Basis of Singwi-Tosi-Land-Sjölander Approximation

Shigenori Tanaka*

*Graduate School of System Informatics, Kobe University,*

*1-1 Rokkodai, Nada, Kobe 657-8501, Japan*

*Electronic address: `tanaka2@kobe-u.ac.jp`

## I. INTERACTION ENERGIES IN THE FERROMAGNETIC STATE

The interaction energies of electron fluid calculated in the Singwi-Tosi-Land-Sjölander (STLS) approximation are listed as functions of $\theta$ and $\Gamma$ in the ferromagnetic ($\zeta = 1$) state. Table S1 below shows the results for negative of interaction energy per particle in units of $e^2/a$, $-\varepsilon_{int}$. Concerning the results for the paramagnetic state, see the literature [1].


[1] S. Tanaka and S. Ichimaru, J. Phys. Soc. Jpn. **55**, 2278 (1986).

TABLE S1. The STLS results for $-\varepsilon_{int}$ in the ferromagnetic state.

| $\theta$ | $\Gamma$ | $-\varepsilon_{int}$ | $\theta$ | $\Gamma$ | $-\varepsilon_{int}$ | $\theta$ | $\Gamma$ | $-\varepsilon_{int}$ |
|---|---|---|---|---|---|---|---|---|
| 0.1 | 0.01 | 0.56740 | 1.0 | 0.01 | 0.34993 | 5.0 | 0.001 | 0.10422 |
| 0.1 | 0.02 | 0.56846 | 1.0 | 0.02 | 0.36703 | 5.0 | 0.002 | 0.11453 |
| 0.1 | 0.05 | 0.57060 | 1.0 | 0.05 | 0.39889 | 5.0 | 0.005 | 0.13469 |
| 0.1 | 0.1 | 0.57305 | 1.0 | 0.1 | 0.43174 | 5.0 | 0.01 | 0.15693 |
| 0.1 | 0.2 | 0.57660 | 1.0 | 0.2 | 0.47310 | 5.0 | 0.02 | 0.18750 |
| 0.1 | 0.5 | 0.58394 | 1.0 | 0.5 | 0.53996 | 5.0 | 0.05 | 0.24487 |
| 0.1 | 1.0 | 0.59255 | 1.0 | 0.7 | 0.56692 | 5.0 | 0.1 | 0.30392 |
| 0.1 | 2.0 | 0.60506 | 1.0 | 1.0 | 0.59596 | 5.0 | 0.2 | 0.37696 |
| 0.1 | 5.0 | 0.62950 | 1.0 | 2.0 | 0.65047 | 5.0 | 0.5 | 0.48841 |
| 0.1 | 10.0 | 0.65434 | 1.0 | 3.0 | 0.67907 | 5.0 | 0.7 | 0.53020 |
| 0.1 | 20.0 | 0.68292 | 1.0 | 4.0 | 0.69718 | 5.0 | 1.0 | 0.57292 |
| 0.1 | 30.0 | 0.69999 | 1.0 | 5.0 | 0.70983 | 5.0 | 1.5 | 0.61793 |
| 0.1 | 50.0 | 0.72037 | 1.0 | 6.0 | 0.71923 | 5.0 | 2.0 | 0.64683 |
| 0.1 | 70.0 | 0.73255 | 1.0 | 7.0 | 0.72653 | 5.0 | 2.5 | 0.66729 |
| 0.1 | 100.0 | 0.74411 | 1.0 | 8.0 | 0.73239 | 5.0 | 3.0 | 0.68268 |
| 0.1 | 120.0 | 0.74947 | 1.0 | 9.0 | 0.73721 | 5.0 | 3.5 | 0.69474 |
| 0.1 | 150.0 | 0.75551 | 1.0 | 10.0 | 0.74126 | 5.0 | 4.0 | 0.70450 |
| 0.1 | 200.0 | 0.76250 | 1.0 | 12.0 | 0.74771 | 5.0 | 4.5 | 0.71257 |
| 0.1 | 220.0 | 0.76463 | 1.0 | 15.0 | 0.75472 | 5.0 | 5.0 | 0.71937 |
| 0.1 | 250.0 | 0.76734 | 1.0 | 20.0 | 0.76249 | 5.0 | 5.5 | 0.72520 |
| 0.1 | 270.0 | 0.76890 | 1.0 | 25.0 | 0.76767 | 5.0 | 6.0 | 0.73025 |
| 0.1 | 280.0 | 0.76962 | 1.0 | 30.0 | 0.77143 | 5.0 | 6.5 | 0.73468 |
| 0.1 | 290.0 | 0.77030 | 1.0 | 40.0 | 0.77663 | 5.0 | 7.0 | 0.73859 |
| 0.1 | 300.0 | 0.77095 | | | | | | |
